# Supplementary material for: Sequence alignment, mutual information, and dissimilarity measures for constructing phylogenies
Source: arXiv:1008.3358 ancillary file (2010-08-19)
Supplement: Supplementary file 1 [file newSI_final.pdf]

# Supplementary Material

## Sequence alignment, mutual information, and dissimilarity measures for constructing phylogenies

O. Penner, P. Grassberger, and M. Paczuski

1) Mutual information (MI) provides in principle an absolute and objective measure of the similarity between any two sequences $A$ and $B$ built from a finite alphabet. It is, however, not easily estimated – and not entirely without any model assumptions such as absence of long range correlations or optimality of compression algorithms. MI estimates can be obtained by means of Shannon information theory or via algorithmic complexity. We first discuss the latter method and turn to Shannon theory in our discussion of quartets. A main result of our paper is that MI can be estimated from alignments in general, and from *global* alignments in particular. This is done by first using an alignment between $A$ and $B$ to construct two 'translation strings', $T_{B|A}$ and $T_{A|B}$, which allow to reconstruct uniquely $B$ from $A$ and $A$ from $B$, respectively. After compression, the lengths of these strings give estimates of the conditional algorithmic informations $K(B|A)$ and $K(A|B)$. Finally, the (algorithmic) MI is estimated by means of the general relations [1]

$$I(A;B) = K(A) - K(A|B), \quad I(B;A) = K(B) - K(B|A), \tag{1}$$

where $K(A)$ and $K(B)$ are the algorithmic informations (also called "Kolmogorov-Chaitin complexities") of the sequences $A$ and $B$. These are estimated by the lengths of compressed versions of $A$ and $B$. A central result of algorithmic information theory is that $I(A;B) = I(B;A)$ up to terms $O(\log N)$, where $N$ is the length of the concatenation $AB$ [1].

The mutual informations estimated this way, denoted $I_{\rm align}$ (see Eq. (3)), can be compared to estimates of MI obtained without using any alignment. The latter can be obtained by comparing the combined lengths of the compressed versions of $A$ and $B$ to the length of a compressed version of the concatenation $AB$. We denote this $I_{\rm compr}$ and it is given by Eq. (4). An unexpected result of the present paper is that both estimates, in spite of being independent and following rather different strategies, yield very similar results for mitochondrial DNA (mtDNA) of vertebrates. More precisely, they give practically *identical* estimates for species within the same family. $I_{\rm align}$ is typically slightly larger for species in the same class but in different families, while $I_{\rm compr}$ is larger for species in different phyla, a case where global alignment algorithms break down.

2) The estimate $I_{\rm compr}$ is the standard estimate for the MI between two strings, and has been used recently in a large number of biological and non-biological problems [2–6]. Most of the work done with $I_{\rm compr}$ has focused on

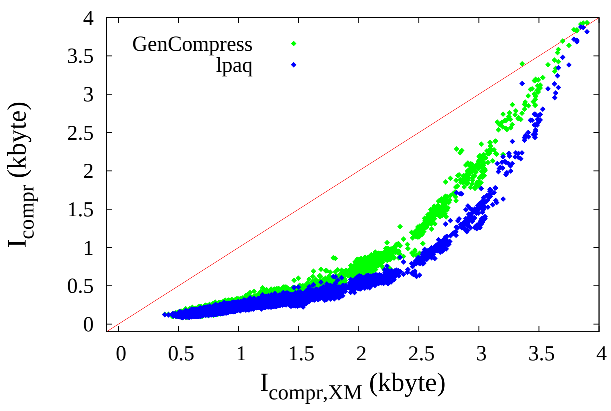


FIG. 1: Scatter plot comparing MI estimates $I_{\rm compr}$ obtained with different compression algorithms, for complete mammalian mtDNA. Note that XM produces higher and, hence, better estimates of $I_{\rm compr}$ than both GenCompress and lpaq1. In addition to lpaq1 we also tested dark, bbb, paq9, paq8, and durilca [9]. The results for all of these algorithms are qualitatively the same as those shown for lpaq1.

clustering of sequences and building phylogenetic trees, however it seems that this activity has met with considerable skepticism in the biological community. One reason is that it seems as if no biological knowledge is incorporated to estimate $I_{\rm compr}$. This is in stark contrast to the substantial amount of biological exertise that goes into constructing phylogenies based on alignments. Another concern is that the value of $I_{\rm compr}$ depends on the quality of the compression algorithm. While two compression algorithms can be easily compared via the lengths of the compressed files they produce, it is impossible to judge the quality of a compression algorithm on an absolute scale. Most non-trivial sequences like DNA, proteins, music, or written language show long range and structurally complex correlations. To obtain good estimates of $I_{\rm compr}$ it is crucial to take these long range effects into account. However, their precise structure and their affect on compressibility are usually not known.

A last reason why compression based methods in phylogeny have been viewed critically is that the MI-based distance measures used in [2–6] are not *additive* (or "tree metrics"), i.e. they do not satisfy the four-point condition [7]. According to [3, 4], the preferred distance is the *normalized compression distance* $d^{\rm (NCD)}$ defined in Eq.(9). Instead of increasing linearly with evolutionary distance, it tends to $d^{\rm (NCD)} = 1$ for maximally distinct pairs. This is considered a severe drawback in phylogenetic applications, in particular it leads to the phenomenon of 'long branch attraction' [8].

It was accepted, up to the turn of the century, that biosequences (DNA, amino acids) are hardly compressible [10, 11], and work on special compression algorithms for DNA and amino acid sequences began. Although there has been substantial progress during the decade in

general purpose compression algorithms, we found that still none of the general purpose algorithms we checked (lpaq1, durilca, bbb, dark [9]) gave better compression for DNA than GenCompress [2] – one of the best public domain DNA compression algorithm available prior to 2007. But the latter also gives poor compression rates, and it was not clear whether this is an inherent problem of DNA or due to weaknesses of the algorithms.

The situation has changed substantially with the development of XM [12], which gives unambigously better results than previous algorithms. According to the authors of Ref. [12], the improvement brought by XM over previous DNA compression algorithms (such as GenCompress) is only a few per cent, when single sequences are considered. However, we found that the improvement in estimates of $I_{\rm compr}$ is much larger for concatenated pairs, presumably because long range correlations and approximate repetitions – which are better captured by XM – play a much larger role.

Results for $I_{\rm compr}$ using GenCompress and lpaq1 versus $I_{\rm compr}$ using XM are shown in Fig. S1. We observe vast differences, except for very closely related species, where all three compression algorithms detect the strong similarity. For species in different families, XM gives typically three to five times larger MIs than GenCompress. Note that we do not have a rigorous proof that larger values of $I_{\rm compr}$ are more accurate. The difficulty is that $I_{\rm compr}$ is the difference between terms which are all overestimated. But the negative term, corresponding to $K(AB)$, is the most difficult to estimate and hence the most likely to be strongly overestimated. As such, it follows that larger values of $I_{\rm compr}$ indicate improved treatment of long-range interdependencies and better MI estimates.

The very strong dependence on compression algorithm observed in Fig. S1 seems to justify skepticism against the use of $I_{\rm compr}$. This is contradicted, however, by the fact that the values of $I_{\rm compr}$ obtained with XM are in very good general agreement with the values of $I_{\rm align}$, as shown in Fig. 2 of the main paper. The latter suggests that it should be possible to improve $I_{\rm compr}$ further by a factor $\approx 1.5$ for species in different classes and by $\approx 2$ for species in different phyla, but probably not by more.

3) As pointed out in the main text, one can estimate the conditional complexity of a sequence $B$, conditioned on another sequence $A$, by simply compressing the translation string $T_{B|A}$. This would give Eq.(1), and it would be the best possible estimate if $T_{B|A}$ were independent $A$. This is certainly a reasonable first approximation, but to check it we estimated the MI between $T_{B|A}$ and $A$ for a large number of mtDNA pairs. Notice that this MI is precisely – up to corrections of order $\log(N)$ and up to the uncertainties of estimating MI using a given compression algorithm – the difference between Eqs.(2) and (1). Results are shown in Fig. S2. They show that correlations between translation and conditioning sequences are in all cases small and could have been neglected without introducing large errors. They have a tendency to

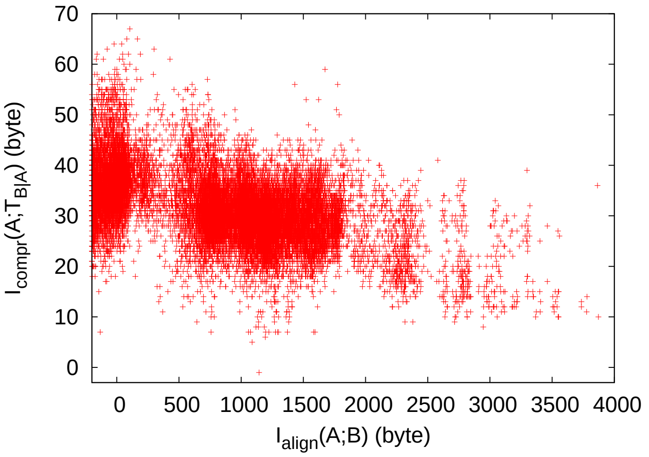


FIG. 2: Scatter plot of mutual informations between translation strings $T_{B|A}$ and conditioning strings $A$, versus the MI between $A$ and $B$. Both values are estimated via compression with lpaq1. The plot uses the same mtDNA pairs as Figure 2.

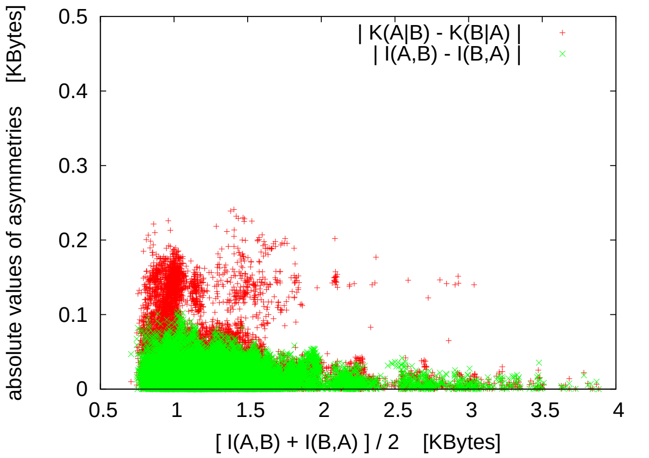


FIG. 3: Scatter plot of asymmetries of $I_{\rm align}$ and of conditional informations, both versus $I_{\rm align}$. In contrast to the previous figures, this plot involves only mammals.

decrease with increasing $I_{\rm align}(A;B)$.

4) An important aspect of our treatment is that the translation strings $T_{B|A}$ and $T_{A|B}$ are different, as long as they contain indels. Thus the conditional informations $K(B|A)$ and $K(A|B)$ are also different. This is in stark contrast to the notion of edit distances, where one typically defines a symmetric distance measure directly via the number and costs of edit operations. In our case the symmetric distance is obtained by first estimating MIs and then by deriving compression distances from them [3]. Although this appears more complicated, it has the advantage of providing a direct link with information theory.

A crucial requirement for our formalism is that the estimates $I_{\rm align}$ should be symmetric under the exchange of the sequences within terms of $O(\log N)$, $I(A;B)_{\rm align} \approx$

```
A     GGGAGATATAGCCGTTATGTGAATAGCACTGAATCAAGCGGCGTACGCGTTATGTGA
B

A'    GGGAGATATAGCCGTTATGTGAATAGCACTGAATCAAGCGGCGTACGCGTTATGTGA
B'    ---------------------------------------------------------
TA|B  GGGAGATATAGCCGTTATGTGAATAGCACTGAATCAAGCGGCGTACGCGTTATGTGA
TB|A  ---------------------------------------------------------
```

FIG. 4: Alignment and translation strings for comparing a random sequence with an empty one. Here, sequence $A$ is random of length $n$, while $B$ is empty. As explained in the text, the estimated MIs $I(B;A)_{\rm align}$ and $I(A;B)_{\rm align}$ agree with the expected results within terms of order $\mathcal{O}(\log n)$.

```
A     GGGCGCTCTCGAAGTTCTGTGCCTAGTT
B     CCCCCCCCCCCCCCCCCCCCCCCCCCCC

A'    GGGCGCTCTCGAAGTTCTGTGCCTAGTT----------------------------
B'    ----------------------------CCCCCCCCCCCCCCCCCCCCCCCCCCCC
TA|B  GGGCGCTCTCGAAGTTCTGTGCCTAGTT----------------------------
TB|A  ----------------------------CCCCCCCCCCCCCCCCCCCCCCCCCCCC
```

FIG. 5: Alignment and translation strings for comparing a random sequence with a sequence composed of only one letter. Here, $A$ is a random sequence of length $n$, while $B$ is a string of $n$ letters "C". As explained in the text, the estimated MIs $I(B;A)_{\rm align}$ and $I(A;B)_{\rm align}$ again agree with the expected results within terms of order $\mathcal{O}(\log n)$.

$I(B;A)_{\rm align}$. Any strong violation of this symmetry would indicate that either the construction of the translation string is not optimal, or that the compression algorithm used in Eq. (3) is deficient. In contrast it is not required that $K(B|A)$ is symmetric. To show that $I(A;B)_{\rm align}$ is more symmetric than $K(B|A)$, we plot in Fig. S3 the differences $|I(A;B)_{\rm align} - I(B;A)_{\rm align}|$ and $|K(B|A) - K(A|B)|$ against $I(A;B)_{\rm align}$. Here we consider only mammalian mtDNA, because the estimates $I(A;B)_{\rm align}$ for species in different classes are too uncertain for a meaningful analysis. We see that there are no problems at all for closely related species, as in such cases both $I(A;B)_{\rm align}$ and $K(B|A)$ are symmetric. For more distant species, both are still symmetric for the majority of pairs, but there are also numerous outliers where $K(B|A)$ is strongly asymmetric. In all those cases the asymmetry of $I(A;B)_{\rm align}$ is significantly smaller than that of $K(B|A)$.

5) In the main text we argued how the symmetry of $I(A;B)_{\rm align}$ is compatible with asymmetric values of $K(B|A)$. Here we shall present some exact results for some extreme cases.

a) Assume that string $A$ is a random string, of length $n$, over the alphabet $\{A,C,G,T\}$ and $B$ is the empty string. Then the optimal alignment is shown in Fig. S4. In order to specify $T_{B|A}$ one must encode the letter "-" and the number $n$ of repetitions, giving $K(B|A) \approx \log_2 n$ bits. On the other hand, $K(A|B) = K(A)$. These give $I(B;A)_{\rm align} \approx -\log_2 n$ bits and $I(A;B)_{\rm align} = \mathcal{O}(1)$. The reason why $I(A;B)_{\rm align}$ is not exactly zero is that the two terms on the r.h.s. of Eq. (3) are compressed using different algorithms. Both have to be specified verbatim, so the only difference between the two term in Eq. (3) is the difference between the overheads in lpaq1 and XM.

```
A     CCCTCCCCGCCCACCCCTCCCCCGCCAA
B     CCCCCCCCCCCCCCCCCCCCCCCCCCCC

          Alignment 1
A'    CCCTCCCCGCCCACCCCTCCCCCGCCAA
B'    CCCCCCCCCCCCCCCCCCCCCCCCCCCC
TA|B  0001000030002000010000030022
TB|A  0001000030002000010000030022

          Alignment 2
A'    CCCTCCCCGCCCACCCCTCCCCCGCCAA----------------------------
B'    ----------------------------CCCCCCCCCCCCCCCCCCCCCCCCCCCC
TA|B  CCCTCCCCGCCCACCCCTCCCCCGCCAA----------------------------
TB|A  ----------------------------CCCCCCCCCCCCCCCCCCCCCCCCCCCC
```

FIG. 6: Two alternative alignments between a biased random sequence and a sequence composed of only one letter. See the text for details.

In summary, $I(B;A)_{\rm align} - I(A;B)_{\rm align} = O(\log n)$, as expected on general grounds for the difference between the exact MI values.

b) Assume that $A$ is as in the above case, and $B$ a string of the same length consisting of a single letter, say "C". The optimal alignment for this case is shown in Fig. S5. Now $T_{B|A}$ consists of $n$ hyphens followed by $n$ "C"s, which gives $I(B;A)_{\rm align} \approx -\log_2 n$ bits. Similarly, $T_{A|B} = A$, followed by $n$ hyphens, so that also $I(A;B)_{\rm align} \approx -\log_2 n$. Thus, for Fig. S5 the difference $I(B;A)_{\rm align} - I(A;B)_{\rm align}$ is again as expected for the exact MI values.

c) Finally, we can consider a situation similar to case b), but with $A$ not fully random. Instead, we assume that $A$ is iid. with prob$(A_i = {\rm C}) \gg$ prob$(A_i = {\rm A}) =$ prob$(A_i = {\rm G}) =$ prob$(A_i = {\rm T})$. In this case one might be inclined intuitively to prefer alignment #1 of Fig. S6 over alignment #2. But for alignment #1 both $T_{B|A}$ and $T_{A|B}$ would be equal to $A$, up to a complexity preserving transformation A→1, C→0, G→3, and T→2. Thus $I(B;A)_{\rm align} \propto n$, while $I(A;B)_{\rm align} = \mathcal{O}(1)$. On the other hand, for alignment #2 both $I(B;A)_{\rm align}$ and $I(A;B)_{\rm align}$ are the same as in Fig. S5. Thus alignment #2 is the optimal alignment, although one might have preferred alignment #1 intuitively.

6) Up to now, we have assumed that the two DNA files contain only the four letters "A", "C", "G", and "T". In reality, the data banks allow also for "wild card" letters indicating ambiguities: "N" for any nucleotide, "R" for a purine, "Y" for a pyrimidine, etc. [13]. Whenever either of the two sequences contains such a wild card character, we put $T_{B|A,i} = B_i$, i.e. the letter in the target string is copied verbatim. This will in some cases slightly overestimate the conditional information $K(B|A)$. But such overdestimations are expected to occur anyhow, and in the data base we used, wild cards are sufficiently rare to have very little effect.

7) In the case of proteins (i.e. amino acid sequences) we have an alphabet of 20 letters. This makes the analysis a bit more lengthy, although it is otherwise the same as for DNA. The translation strings now contains 41 characters: Twenty letters for specifying insertions, one hyphen for indicating a deletion, and 20 numbers for indicating

```
A'      GGGAG---ATATAGCCGTTATGTGAATAGCACTGAATCAAGCG---------GCGT
B'      GGGAC---ATATAG----TATGTAAATATCACTGAATCGAACGAACACGCACGTGT
C'      GGGACGGGATATAGCCGTTATGTAA-----ACTGTATCAAGCGAACACGCACGTGT
T_C|A,B 00003GGG000000C0000000010-----0000300010000A000000000000
```

FIG. 7: Alignment of a third sequence $C$ to an already existing alignment between $A$ and $B$. The translation string $T_{C|AB}$ for reconstructing $C$ from $A$ and $B$ is obtained by using locally one of the strings $A$ and $B$ as "master strings" and applying the rules described in the main part of the paper. The actual master string is printed in red.

substitutions. For the latter we have some freedom. As for DNA, we could encode forward and backward substitutions by the same number. Apart from that, we could use this freedom in the case of amino acids also to optimally encode substitutions. This optimization would likely rely on PAM or similar matricies. Alternatively, we could encode the 20 amino acids by numbers $0 \ldots 19$, and encode a substitution $j \to k$ $(j, k = 0 \ldots 19)$ by the number $k - j \mod 20$. This has the advantage of simplicity, but led in the case of DNA to marginally worse results.

8) For local alignments, the output of an alignment algorithm consists of a list of matching regions, together with the actual alignments of those regions. These matching regions can in principle overlap. Thus in order to construct $T_{B|A}$, one first has to select a subset of matching regions $\mathcal{M}_k$ that do not overlap on sequence $B$. Each one of these matches is characterized by its starting points in sequences $A$ and $B$ and by the translation string restricted to the matching regions,

$$\mathcal{M}_k \equiv \{n_k^{(A)}, n_k^{(B)}, T_{B|A;k}\}. \tag{2}$$

The entire translation string consists of all these pieces of information, separated by uniquely decodable separators, plus the verbatim description of sequence $B$ in regions where no matches were found or used. Indeed, if one has the latter verbatim description and all translation strings $T_{B|A;k}$ for the matching regions, one can recover the points $n_k^{(B)}$ and does not have to include them in $T_{B|A}$ explicitly.

9) As a first step towards multiple alignments we discuss the alignment of a sequence $C$ to an already existing and fixed alignment of two sequences $A$ and $B$, and the corresponding MI estimate $I(C;(A,B))_{\rm align}$. An application of this could be to estimate the similarity between mouse and the family of hominides, where the latter is characterised by the two species homo and chimpanzee. The central problem is to construct a translation string which allows to reconstruct $C$ from the aligned pair $(A, B)$.

One possibility is illustrated in Fig. S7. We start at position $i = 1$ and construct $T_{C|AB}$ from left to right, using at each step one of the sequences $A$ or $B$ as the "master sequence". If $A$ is presently the master sequence, then $T_{C|AB,i} = T_{C|A,i}$, where $T_{C|A,i}$ is as described in the main paper. Similarly, if $B$ is the master sequence, then $T_{C|AB,i} = T_{C|B,i}$. The status of master sequence is kept until $C'_i$ disagrees with the character in the master sequence *and* is identical to the character in the other (non-master) sequence, at which point master and non-master sequences switch their status. In a slightly more sophisticated version, one keeps track of the number of 'mistakes' made recently by sequences $A$ and $B$, and switches only when the current master has done worse over the recent past. We have no proof that either encoding is optimal, but both guarantee at least that the "better" of the two sequences $A$ and $B$ is used as a template to reconstruct $C$.

We note estimating $I(C;(A,B))$ via concatenation and compression alone is easy. One just has to modify Eq. (4) to

$$\begin{aligned} I(C;(A,B))_{\rm compr} &= {\rm len}[{\rm XM}(AB)] + {\rm len}[{\rm XM}(C)] \\ &- {\rm len}[{\rm XM}(ABC)], \end{aligned} \tag{3}$$

where $AB$ and $ABC$ denote the concatenations of $A$ with $B$ and of $AB$ with $C$. This gives $I(C;(A,B))_{\rm compr} \geq I(C;A)_{\rm compr}$ and $I(C;(A,B))_{\rm compr} \geq I(C;B)_{\rm compr}$, in agreement with general relations between MIs and with intuition. In contrast, concatenating $A$ and $B$ and then aligning (globally!) $C$ with $AB$ would lead to very poor estimates of $I(C;(A,B))_{\rm align}$.

We have made preliminary numerical tests showing that the proposals in points 6) to 8) are potentially feasible, but more complete investigations are needed and will be presented in future publications.

10) **Definition of significances for quartets**

For any quartet of sequences $A, B, C$ and $D$, we first measure the distance matrix $d_{ij}$ with $i, j \in \{A, B, C, D\}$. If these distances satisfy the four-point condition, we obtain

$$\begin{aligned} b &\equiv \frac{1}{2} \max\min\{d_{ij} + d_{kl} - d_{ik} - d_{jl}, d_{ij} + d_{kl} - d_{il} - d_{jk}\} \\ &= 0, \end{aligned} \tag{4}$$

where the maximum is over all permutations $(A, B, C, D) \to (i, j, k, l)$ and the minimum is, for each permutation, over the two terms in the curly bracket. If $b > 0$, the four-point condition is violated. A second quantity of interest is

$$a \equiv \frac{1}{2} \max(d_{ij} + d_{kl} - d_{ik} - d_{jl}) \ . \tag{5}$$

Where the maximum is over permutations of the indicies. Obviously, $b \leq a$.

If $b = 0$, i.e. if the distances can be exactly represented by an (unrooted) tree, then $a$ is the length of the central edge. If not, the distances cannot be represented by a tree, but by the most simple example of a *split graph* [14]: A graph consisting of a parallelepiped in the center and four legs connecting to the leaves $A$ to $D$. The two quantities $a$ and $b$ are the lengths of the two edges of the parallelepiped. If $b = a$ the inner box is a rhombus

and no partitioning of the quartet into pairs $((ij)(kl))$ is preferred. Thus we take $a-b$, after normalizing it properly, as a significance measure,

$$S = \frac{2(a-b)}{\max\{d_{ik}+d_{jl}, d_{il}+d_{jk}\}} \ . \qquad (6)$$

The preferred partition is that for which $d_{ik}+d_{jl}-d_{ij}-d_{kl} > 2b$. The significance is bounded by $0 \leq S \leq 1$.

11) **Most significant disagreements for topologies based on $d^{(\log-\mathrm{det})}, d^{(\log-\mathrm{MI})}$, and $d^{(\mathrm{NSD})}$**

If two metrics predict different topologies 1 and 2 with significances $S_1$ and $S_2$, then we define the significance of the disagreement as $S_{12} = S_1 + S_2$. A list of quartets that contain some of the most significant clashes between $d^{(\log-\mathrm{det})}$ and $d^{(\log-\mathrm{MI})}$ are found in Tables S1 to S9, with the somewhat unsystematic selection criteria discussed in the main text. We should stress, however, that the selection – which was made to minimize clustering of quartets in few taxa – was done blindly, i.e. by representing species by numbers and avoiding triplets that occur more than once in the list.

Clashes between $d^{(\log-\mathrm{MI})}$ and $d^{(\mathrm{NSD})}$ were fewer – less than half of those between $d^{(\log-\mathrm{det})}$ and $d^{(\log-\mathrm{MI})}$ – and had smaller significances. The largest values of $S_{ij}$ were typically only half of the largest $S_{ij}$ for $d^{(\log-\mathrm{det})}$ and $d^{(\log-\mathrm{MI})}$, for each clade. The smaller significances together with generally poor agreement in the literature, as to the "true" groupings, suggests that these clashes are of less biological significance, and we do not list them.

12) **Definition of two distance measures based on the 2-parameter Kimura model**

In Kimura's model [15] it is assumed that transitions (A↔ G, C↔T) and transversions (A↔ C, G↔T,A↔ T, C↔G) have different rates $\alpha$ and $\beta$. For fixed $\alpha$, $\beta$, and evolution time $t$, the log-likelihood for observed substitution frequencies $f_{AB}(i,k)$ is [16] (p. 230)

$$L_{AB} = m_{\mathrm{ident}} \log r + m_{\mathrm{transi}} \log s + m_{\mathrm{transv}} \log u, \qquad (7)$$

where $m_{\mathrm{type}}$ is the number of observed types of "substitutions", $s = (1-e^{-4\beta t})/4$, $u = (1-e^{-4\beta t} - 2e^{-2(\alpha+\beta)t})/4$, and $r = 1-2s-u$. Notice that when we assume $\beta$ and $\alpha$ are drawn from a model (as opposed to fitting) this is reminiscent of a Kullback-Leibler [1] version of MI,

$$L_{AB} = \frac{1}{M} \sum_{i,j\in\{A,C,G,T\}} f_{AB}(i,j) \log \frac{Q_{ij}}{Q_i Q_j} - \log 4.$$

Here $M$ is the lenght of the sequences, $\mathbf{f}_{AB}$ is the observed substitution matrix, $\mathbf{Q}$ is the substitution matrix of the model,

$$\mathbf{Q} = \begin{pmatrix} r & s & u & s \\ s & r & s & u \\ u & s & r & s \\ s & u & s & r \end{pmatrix} \ , \qquad (8)$$

and the equilibrium distribution of the model is $\vec{Q} = (1/4, 1/4, 1/4, 1/4, 1/4)$. For given $m_{\mathrm{type}}$, the likelihood is maximal if $u = m_{\mathrm{transi}}$, $s = m_{\mathrm{transv}}/2$, and $r = m_{\mathrm{ident}}$, which in turn gives values for $\alpha t$ and $\beta t$.

The most natural *a priori* candidate for a distance in the Kimura model is the absolute value of $L$ itself,

$$d_{AB}^{(\mathrm{Kimura}_1)} = -L_{AB}. \qquad (9)$$

This is, however, *not* what is commonly used. Rather, the *Kimura distance* is defined as the average total number of substitutions, including the "hidden" ones, which is

$$d_{AB}^{(\mathrm{Kimura}_2)} = (\alpha+2\beta)t = -\frac{1}{2}\log\frac{m_{\mathrm{ident}} - m_{\mathrm{transi}}}{M} - \frac{1}{4}\log\frac{m_{\mathrm{ident}} + m_{\mathrm{transi}} - m_{\mathrm{transv}}}{M}. \qquad (10)$$

Although this distance has the advantage of being additive, it has serious drawback: Given that transitions and transversions occur at different rates, it does not seem to make much sense to taken an unweighted sum over both as a distance measure.

13) **An example of quartet misclassification due to metric non-addivity**

We discuss here the quartet formed by three Ursus species (*U. maritimus, U. americanus*, and *U. thibetanus*) and a Lagomorph species (*Orcytolagus cuniculus*). According to [41], the grouping of the three Ursidae is ((*maritimus, americanus*), *thibetanus*). The two distance matrices obtained with $d^{(\mathrm{NSD})}$ and with $d^{(\log-\mathrm{MI})}$ (i.e. with the original and the log-transformed versions of the Shannon-MI based distances) are shown in Table 10. We see that the smallest distance is between *U. americanus* and *U. thibetanus* Hence, the evolutionary speeds within the Ursidae must have been different. Using $d^{(\mathrm{NSD})}$, the outgroup species (*O. cuniculus*) has roughly the same distances from all three (because they are already close to saturation, as expected for a distant outgroup and a metric where distances converge to a finite value when evolutionar distances tend to infinity), and thus the Felsenstein phenomenon gives the wrong grouping ((*americanus, thibetanus*), *maritimus*). What is no longer true after log-transforming, as this increases the distance differences to the outgroup species. But since these differences are affected by amplified random errors, the resulting grouping ((*maritimus, thibetanus*), *americanus*) is also wrong.

Note that this example is better called "small distance attraction", in contrast to the "large distance attraction" observed in standard textbook examples of the Felsenstein phenomenon. The latter is due to the fact that in these examples *two* species are distant from the other two, while in our example only one is distant from the other two. But the basic reason for the misclassification is the same, and "large distance" attraction is indeed at the same time also a "small distance" attraction. We chose our example for more intuitive interpretation.

[1] T. Cover and J. Thomas, *Elements of information theory* (John Wiley & Sons, Hoboken, 2006), 2nd ed.

[2] M. Li, J. Badger, X. Chen, S. Kwong, P. Kearney, and H. Zhang, Bioinformatics **17**, 149 (2001).

[3] M. Li, X. Chen, X. Li, B. Ma, and P. Vitanyi, IEEE Trans. Inf. Theory **50**, 3250 (2004).

[4] R. Cilibrasi and P. Vitanyi, IEEE Trans. Inf. Theory **51**, 1523 (2005).

[5] A. Kraskov, H. Stoegbauer, R. Andrzejak, and P. Grassberger, Europhysics Letters **70**, 278 (2005).

[6] A. Kraskov and P. Grassberger, *Mic: Mutual information based hierarchical clustering* (2008).

[7] W. Press, S. Teukolski, W. Vetterling, and B. Flannery, *Numerical Recipes, 3rd edition* (Cambridge University Press Cambridge, 2007).

[8] J. Felsenstein, J. Mol. Evol. **17**, 368 (1981).

[9] *http://cs.fit.edu/~mmahoney/compression/text.html* (2008).

[10] S. Grumbach and F. Tahi, DCC pp. 340–350 (1993).

[11] *http://monod.uwaterloo.ca/downloads/gencompress/* (2003).

[12] M. Cao, T. Dix, L. Allison, and C. Mears, Proceedings of the 2007 Data Compression Conference pp. 43–52 (2007).

[13]

[14] H. Bandelt and A. Dress, Molecular Phylogenetics and Evolution **1**, 242 (1992).

[15] (????).

[16] R. Durbin, S. Eddy, A. Krogh, and G. Mitchison, *Biological sequence analysis: Probabilistic models of proteins and nucleic acids* (Cambridge University Press Cambridge, 1998).

[17] Y. Kitazoe, H. Kishino, P. Waddell, N. Nakajima, T. Okabayashi, T. Watanabe, and Y. Okuhara, PLoS one **2**, e384 (2007).

[18] G. Wesley-Hunt and J. Flynn, Journal of Systematic Palaeontology **3**, 1 (2005).

[19] J. Flynn, J. Finarelli, S. Zehr, J. Hsu, and M. Nedbal, Systematic Biology **54**, 317 (2005).

[20] J. Nelson, *Fishes of the World* (John Wiley, New York, 2006), 4th ed.

[21] C. Li, Ph.D. thesis, University of Nebraska (2007).

[22] W. Chen, C. Bonillo, and G. Lecointre, Molecular Phylogenetics and Evolution **26**, 262 (2003).

[23] P. Gaubert, G. Denys, and T. Oberdorff, Biological Reviews **84**, 653 (2009).

[24] *http://tolweb.org/Neoptera/8267* (2003).

[25] *http://www.ncbi.nlm.nih.gov/Taxonomy/Browser/wwwtax.cgi?mode=Und.*

[26] S. Cameron, C. Lambkin, S. Barker, and M. Whiting, Systematic Entomology **32**, 40 (2006).

[27] *http://en.wikipedia.org/wiki.*

[28] T. Engstrom, H. Shaffer, and W. McCord, Syst. Biol. **53**, 693 (2004).

[29] R. Pratt, G. Gibb, M. Morgan-Richards, M. Phillips, M. Hendy, and D. Penny, Mol. Biol. Evol. **26**, 313 (2009).

[30] S. Eo, Zoologica Scripta **38**, 465 (2009).

[31] *http://tolweb.org/Caudata/14939* (2006).

[32] R. Mueller, J. Macey, M. Jaekel, D. Wake, and J. Boore, Proc. Natl. Acad. Sci. U.S.A. **101**, 13820 (2004).

[33] A. Jex, R. Hall, T. Littlewood, and R. Gasser, Nucleic Acids Research **38**, 522 (2010).

[34] Y. Liu and Z. Cui, Mol. Biol. Rep. pp. 10.1007/s11033–009–9773–2 (2009).

[35] N. Puillandre, S. Samadi, M. Boiselier, A. Sysoev, Y. Kantor, C. Cruaud, A. Couloux, and P. Bouchet, Molecular Phylogenetics and Evolution **47**, 1122 (2008).

[36] C. Grande, J. Templado, and R. Zardoya, BMC Evol Biol. **8**, 61 (2008).

[37] R. Cunha, C. Grande, and R. Zardoya, BMC Evol Biol. **9**, 210 (2009).

[38] A. Lavikainen, V. Haukisalmi, M. Lehtinen, H. Henttonen, A. Oksanen, and S. Meri, Parasitology **135**, 1457 (2008).

[39] E. Hohberg, Parasitology International **55**, S23 (2006).

[40] M. Nakao, D. McManus, P. Schantz, P. Craig, and A. Ito, Parasitology **134**, 713 (2006).

[41] M. Pagès, S. Calvignac, C. Klein, M. Paris, S. Hughes, and C. Hanni, Molecular Phylogenetics and Evolution **47**, 73 (2008).

| mammals | | | | | | | | | | |
|---|---|---|---|---|---|---|---|---|---|---|
| | species names | | | | | | classification predicted by | | | |
| Nr. | species 1 | species 2 | species 3 | species 4 | "true" | Ref. | $d^{(\log-\mathrm{MI})}$ | $d^{(\log-\det)}$ | $d^{(\mathrm{NSD})}$ | $S_{(\log-\det,\log-\mathrm{MI})}$ |
| 1 | Ursus thibet. thibetanus | Ursus thibetanus | Ursus thibet. mupinensis | Ursus maritimus | ? | – | (12)(34) | (14)(23) | (12)(34) | 0.05719 |
| 2 | Cricetulus griseus | Choloepus didactylus | Manis tetradactyla | Hippopotamus amphibius | (12)(34) | [17] | • | (13)(24) | • | 0.03671 |
| 3 | Cricetulus griseus | Pongo abelii | Manis tetradactyla | Hippopotamus amphibius | (12)(34) | [17] | • | (13)(24) | • | 0.03433 |
| 4 | Erignathus barbatus | Ailuropoda melanoleuca | Nyctereutes procyonoides | Mammuthus primigenius | (12)(34) | [17, 18] | • | (13)(24) | • | 0.03404 |
| 5 | Tremarctos ornatus | Callorhinus ursinus | Nyctereutes procyonoides | Phascogale tapoatafa | (12)(34) | [17, 18] | • | (14)(23) | • | 0.03343 |
| 6 | Spilogale putorius | Ceratotherium simum | Hemiechinus auritus | Ochotona princeps | (12)(34) | [17] | • | (13)(24) | • | 0.03334 |
| 7 | Canis lupus chanco | Physeter catodon | Hemiechinus auritus | Pongo pygmaeus | (12)(34) | [17] | • | (13)(24) | • | 0.03305 |
| 8 | Elaphodus cephalophus | Equus caballus | Hemiechinus auritus | Pongo abelii | (12)(34) | [17] | • | (14)(23) | • | 0.03240 |
| 9 | Ursus thibet. mupinensis | Phocarctos hookeri | Acinonyx jubatus | Balaenoptera omurai | (12)(34) | [17, 18] | • | (14)(23) | • | 0.03220 |
| 10 | Elaphodus cephalophus | Kogia breviceps | Martes zibellina | Erinaceus europaeus | (12)(34) | [17] | • | (14)(23) | • | 0.03211 |
| 11 | Hydropotes inermis | Neophoca cinerea | Hemiechinus auritus | Pongo pygmaeus | (12)(34) | [17] | • | (13)(24) | • | 0.03199 |
| 12 | Martes flavigula | Ursus thibet. mupinensis | Capricornis crispus | Spilogale putorius | (12)(34) | [18, 19] | • | (14)(23) | • | 0.03191 |
| 13 | Martes zibellina | Ursus thibet. mupinensis | Acinonyx jubatus | Rhinoceros unicornis | (12)(34) | [18, 19] | • | (13)(24) | • | 0.03173 |
| 14 | Muntiacus crinifrons | Hippopotamus amphibius | Ailuropoda melanoleuca | Ceratotherium simum | (12)(34) | [17] | • | (13)(24) | • | 0.03171 |
| 15 | Manis tetradactyla | Equus caballus | Hemiechinus auritus | Pongo pygmaeus | (12)(34) | [17] | • | (14)(23) | • | 0.03169 |
| 16 | Balaenoptera brydei | Manis tetradactyla | Hemiechinus auritus | Homo sapiens | (12)(34) | [17] | • | (14)(23) | • | 0.03159 |
| 17 | Martes flavigula | Tremarctos ornatus | Stenella attenuata | Canis latrans | (12)(34) | [18, 19] | • | (14)(23) | • | 0.03159 |
| 18 | Canis lupus laniger | Eschrichtius robustus | Hemiechinus auritus | Pongo pygmaeus | (12)(34) | [17] | • | (13)(24) | • | 0.03156 |
| 19 | Martes zibellina | Ursus thibet. thibetanus | Canis lupus chanco | Rhinolophus formosae | (12)(34) | [18, 19] | • | (13)(24) | • | 0.03105 |
| 20 | Martes zibellina | Helarctos malayanus | Canis latrans | Pteropus scapulatus | (12)(34) | [18, 19] | • | (13)(24) | • | 0.03100 |
| 21 | Odobenus rosmar. rosmarus | Eumetopias jubatus | Macroscelides proboscideus | Halichoerus grypus | (12)(34) | [18, 19] | • | (13)(24) | • | 0.03086 |
| 22 | Martes zibellina | Melursus ursinus | Mammut americanum | Felus catus | (12)(34) | [18, 19] | • | (14)(23) | • | 0.02779 |
| 23 | Kogia breviceps | Muntiacus reevesi | Cuon alpinus | Gorilla gorilla | (12)(34) | [17] | • | (14)(23) | • | 0.02640 |

TABLE I: Quartets of mammals for which $d^{(\log-\mathrm{MI})}$ and $d^{(\log-\det)}$ give significantly different classifications. In the last four columns, a bullet means that the correct grouping was predicted with this distance measure; otherwise the predicted grouping is given. Within each quartet, species are arranged so that the the first two are closest according to established taxonomy (whenever available). Quartets are ordered by decreasing significance of the disagreement between log-det and log-MI groupings.

| actinopterygii (ray-finned fish) | | | | | | | | | | |
|---|---|---|---|---|---|---|---|---|---|---|
| | species names | | | | | | classification predicted by | | | |
| Nr. | species 1 | species 2 | species 3 | species 4 | "true" | Ref. | $d^{(\log-\mathrm{MI})}$ | $d^{(\log-\det)}$ | $d^{(\mathrm{NSD})}$ | $S_{(\log-\det,\log-\mathrm{MI})}$ |
| 1 | Bathygadus antrodes | Pterocaesio tile | Anguilla interioris | Albula glossodonta | (12)(34) | [20–22] | • | (14)(23) | • | 0.05574 |
| 2 | Bathygadus antrodes | Thunnus alalunga | Anguilla obscura | Albula glossodonta | (12)(34) | [20–22] | • | (14)(23) | (14)(23) | 0.05296 |
| 3 | Bathygadus antrodes | Caranx melampygus | Anguilla bicolor bicolor | Albula glossodonta | (12)(34) | [20–22] | • | (14)(23) | • | 0.05276 |
| 4 | Bathygadus antrodes | Crenimugil crenilabis | Anguilla japonica | Albula glossodonta | (12)(34) | [20–22] | • | (14)(23) | • | 0.05250 |
| 5 | Bathygadus antrodes | Lophius litulon | Anguilla celebesensis | Albula glossodonta | (12)(34) | [20–22] | • | (14)(23) | • | 0.05226 |
| 6 | Bathygadus antrodes | Ostichthys japonicus | Anguilla dieffenbachii | Albula glossodonta | (12)(34) | [20–22] | • | (14)(23) | • | 0.05200 |
| 7 | Bathygadus antrodes | Dactyloptena tiltoni | Anguilla mossambica | Albula glossodonta | (12)(34) | [20–22] | • | (14)(23) | • | 0.05109 |
| 8 | Bathygadus antrodes | Lates calcarifer | Anguilla obscura | Albula glossodonta | (12)(34) | [20–22] | • | (14)(23) | • | 0.05096 |
| 9 | Spratelloides gracilis | Clupea pallasii | Ilisha elongata | Takifugu ocellatus | (12)(34) | [20] | (14)(23) | • | (14)(23) | 0.03573 |
| 10 | Albula glossodonta | Elops hawaiensis | Nansenia ardesiaca | Galaxias maculatus | (12)(34) | [20, 21] | • | (14)(23) | • | 0.03529 |
| 11 | Ceratias uranoscopus | Eutaeniophorus festivus | Cyema atrum | Gonorynchus greyi | (12)(34) | [20, 21] | • | (14)(23) | • | 0.03277 |
| 12 | Sprattus sprattus | Spratelloides delicatulus | Ilisha africana | Anguilla malgumora | (12)(34) | [20] | (13)(24) | • | (13)(24) | 0.03236 |
| 13 | Clinocottus analis | Fundulus diaphanus | Salangichthys microdon | Puntius ticto | (12)(34) | [20] | • | (13)(24) | • | 0.03114 |
| 14 | Diplacanthopoma brachysoma | Gadus ogac | Parataeniophorus gulosus | Beryx decadactylus | (12)(34) | [20] | • | (14)(23) | • | 0.03032 |
| 15 | Branchiostegus albus | Coreoperca kawamebari | Fundulus diaphanus | Indostomus paradoxus | (12)(34) | [20] | • | (14)(23) | • | 0.02996 |
| 16 | Ceratias uranoscopus | Elassoma evergladei | Salangichthys microdon | Pantodon buchholzi | (12)(34) | [20] | • | (13)(24) | • | 0.02971 |
| 17 | Gila conspersa | Barbus barbus | Psilorhynchus homaloptera | Alepocephalus bairdii | (12)(34) | [23] | • | (13)(24) | • | 0.02965 |
| 18 | Nessorhamphus ingolfianus | Albula glossodonta | Sprattus sprattus | Galaxias maculatus | (12)(34) | [20] | • | (13)(24) | • | 0.02928 |
| 19 | Oryzias sinensis | Diaphus splendidus | Spratelloides delicatulus | Cyema atrum | (12)(34) | [20] | • | (14)(23) | • | 0.02904 |
| 20 | Oncorhynchus clarkii henshawi | Diplophos taenia | Papyrocranus congoensis | Chirocentrus dorab | (12)(34) | [20] | • | (13)(24) | • | 0.02820 |
| 21 | Clinocottus analis | Rudarius ercodes | Barbus trimaculatus | Chirocentrus dorab | (12)(34) | [20] | • | (14)(23) | • | 0.05785 |
| 22 | Fundulus diaphanus | Lagocephalus wheeleri | Eutaeniophorus sp. 033-Miya | Alepocephalus bicolor | (12)(34) | [20] | • | (14)(23) | • | 0.02784 |
| 23 | Oryzias sinensis | Zu cristatus | Alepocephalus bairdii | Albula glossodonta | (12)(34) | [20] | • | (13)(24) | • | 0.02770 |

TABLE II: Same as Table I, but for actinopterygii (ray-finned fishes).

| hexapoda (insects etc.) | | | | | | | | | | |
|---|---|---|---|---|---|---|---|---|---|---|
| | species names | | | | | | classification predicted by | | | |
| Nr. | species 1 | species 2 | species 3 | species 4 | “true” | Ref. | $d^{(\log-\mathrm{MI})}$ | $d^{(\log-\det)}$ | $d^{(\mathrm{NSD})}$ | $S_{(\log-\det,\log-\mathrm{MI})}$ |
| 1 | Reticulitermes santonensis | Periplaneta fuliginosa | Ostrinia nubilalis | Japyx solifugus | (12)(34) | [24, 25] | • | (14)(23) | • | 0.04653 |
| 2 | Reticulitermes flavipes | Periplaneta fuliginosa | Anoplophora glabripennis | Japyx solifugus | (12)(34) | [24, 25] | • | (14)(23) | • | 0.04556 |
| 3 | Reticulitermes santonensis | Periplaneta fuliginosa | Trachypachus holmbergi | Japyx solifugus | (12)(34) | [24, 25] | • | (14)(23) | • | 0.04494 |
| 4 | Reticulitermes virginicus | Periplaneta fuliginosa | Simosyrphus grandicornis | Japyx solifugus | (12)(34) | [24, 25] | • | (14)(23) | • | 0.04478 |
| 5 | Reticulitermes hageni | Periplaneta fuliginosa | Simosyrphus grandicornis | Japyx solifugus | (12)(34) | [24, 25] | • | (14)(23) | • | 0.04414 |
| 6 | Reticulitermes santonensis | Periplaneta fuliginosa | Drosophila sechellia | Japyx solifugus | (12)(34) | [24, 25] | • | (14)(23) | (14)(23) | 0.04400 |
| 7 | Reticulitermes virginicus | Periplaneta fuliginosa | Ostrinia nubilalis | Japyx solifugus | (12)(34) | [24, 25] | • | (14)(23) | • | 0.04252 |
| 8 | Rhopaea magnicornis | Pyrophorus divergens | Coreana raphaelis | Reticulitermes flavipes | (12)(34) | [24, 25] | • | (13)(24) | • | 0.03622 |
| 9 | Pyrophorus divergens | Anoplophora glabripennis | Drosophila sechellia | Reticulitermes hageni | (12)(34) | [24, 25] | • | (14)(23) | (14)(23) | 0.03622 |
| 10 | Reticulitermes santonensis | Periplaneta fuliginosa | Gampsocleis gratiosa | Ostrinia furnacalis | (12)(34) | [24, 25] | • | (13)(24) | • | 0.03444 |
| 11 | Bactrocera oleae | Ceratitis capitata | Drosophila mauritiana | Reticulitermes hageni | (12)(34) | [26] | • | (14)(23) | • | 0.03332 |
| 12 | Reticulitermes santonensis | Simosyrphus grandicornis | Campodea fragilis | Gomphiocephalus hodgsoni | (12)(34) | [24, 25] | • | (13)(24) | • | 0.03269 |
| 13 | Rhopaea magnicornis | Simosyrphus grandicornis | Reticulitermes hageni | Pachypsylla venusta | (12)(34) | [24, 25] | (14)(23) | • | • | 0.03258 |
| 14 | Rhopaea magnicornis | Pyrophorus divergens | Reticulitermes hageni | Simosyrphus grandicornis | (12)(34) | [24, 25] | • | (14)(23) | • | 0.03166 |
| 15 | Gastrimargus marmoratus | Gryllotalpa orientalis | Polystoechotes punctatus | Siphlonurus immanis | (12)(34) | [25, 27] | (13)(24) | • | (13)(24) | 0.03141 |
| 16 | Neuroctenus parus | Drosophila sechellia | Atelura formicaria | Orchesella villosa | (12)(34) | [25, 27] | (13)(24) | (14)(23) | (14)(23) | 0.02949 |
| 17 | Siphlonurus immanis | Davidius lunatus | Reticulitermes flavipes | Ceratitis capitata | (12)(34) | [25, 27] | • | (14)(23) | (14)(23) | 0.02785 |
| 18 | Tetraphalerus bruchi | Sphaerius sp. BT0074 | Atelura formicaria | Onychiurus orientalis | (12)(34) | [25, 27] | • | (13)(24) | • | 0.02545 |

TABLE III: Same as Table I, but for hexapoda (insects etc.).

| sauropsida (reptiles, birds) | | | | | | | | | | |
|---|---|---|---|---|---|---|---|---|---|---|
| | species names | | | | | | classification predicted by | | | |
| Nr. | species 1 | species 2 | species 3 | species 4 | “true” | Ref. | $d^{(\log-\mathrm{MI})}$ | $d^{(\log-\det)}$ | $d^{(\mathrm{NSD})}$ | $S_{(\log-\det,\log-\mathrm{MI})}$ |
| 1 | Trionyx triunguis | Dogania subplana | Lissemys punctata | Polychrus marmoratus | (12)(34) | [28] | • | (13)(24) | • | 0.03026 |
| 2 | Pelodiscus sinensis | Dogania subplana | Lissemys punctata | Indotestudo elongata | (12)(34) | [28] | • | (14)(23) | • | 0.02877 |
| 3 | Pelodiscus sinensis | Dogania subplana | Lissemys punctata | Chinemys reevesi | (12)(34) | [28] | • | (14)(23) | • | 0.02874 |
| 4 | Pelodiscus sinensis | Dogania subplana | Lissemys punctata | Pyxidea mouhotii | (12)(34) | [28] | • | (14)(23) | • | 0.02765 |
| 5 | Trionyx triunguis | Dogania subplana | Lissemys punctata | Cygnus atratus | (12)(34) | [28] | • | (14)(23) | • | 0.02752 |
| 6 | Pterodroma brevirostris | Ciconia ciconia | Tachybaptus novaehollandiae | Anas platyrhynchos | (12)(34) | [29] | • | (13)(24) | • | 0.02706 |
| 7 | Pterodroma brevirostris | Eudyptula minor | Pteroglossus azara flavirostris | Apteryx haastii | (12)(34) | [29] | • | (14)(23) | • | 0.02666 |
| 8 | Lissemys punctata | Dogania subplana | Indotestudo forstenii | Gallus sonneratii | (12)(34) | [25, 27] | (14)(23) | • | (14)(23) | 0.02641 |
| 9 | Tragopan caboti | Syrmaticus ellioti | Gallus varius | Manouria emys | (12)(34) | [30] | • | (13)(24) | • | 0.02623 |
| 10 | Eudyptula minor | Ciconia ciconia | Pteroglossus azara flavirostris | Dromaius novaehollandiae | (12)(34) | [29] | (14)(23) | • | (14)(23) | 0.02573 |
| 11 | Pelodiscus sinensis | Dogania subplana | Lissemys punctata | Cyclemys atripons | (12)(34) | [28] | • | (14)(23) | • | 0.02568 |
| 12 | Tragopan caboti | Syrmaticus humiae | Manouria emys | Dogania subplana | (12)(34) | [25, 27] | • | (14)(23) | • | 0.02435 |
| 13 | Pterodroma brevirostris | Eudyptula minor | Pteroglossus azara flavirostris | Acrocephalus scirpaceus | (12)(34) | [29] | • | (13)(24) | • | 0.02413 |
| 14 | Cathartes aura | Ciconia ciconia | Tachybaptus novaehollandiae | Cairina moschata | (12)(34) | [25, 27] | • | (14)(23) | • | 0.02391 |
| 15 | Pteroglossus azara flavirostris | Dryocopus pileatus | Eudyptula minor | Indotestudo elongata | (12)(34) | [25, 27] | (14)(23) | • | (14)(23) | 0.02378 |
| 16 | Tragopan caboti | Syrmaticus humiae | Gallus gallus gallus | Leiocephalus personatus | (12)(34) | [30] | • | (13)(24) | • | 0.02344 |
| 17 | Phoenicopterus ruber roseus | Cathartes aura | Trogon viridis | Anseranas semipalmata | (12)(34) | [27, 29] | • | (14)(23) | • | 0.02304 |
| 18 | Cuora flavomarginata | Cuora aurocapitata | Pyxidea mouhotii | Syrmaticus humiae | (12)(34) | [25, 27] | (13)(24) | • | (13)(24) | 0.01933 |

TABLE IV: Same as Table I, but for sauropsida (reptiles, birds).

| amphibia | | | | | | | | | | |
|---|---|---|---|---|---|---|---|---|---|---|
| | species names | | | | | | classification predicted by | | | |
| Nr. | species 1 | species 2 | species 3 | species 4 | "true" | Ref. | $d^{(\log-\mathrm{MI})}$ | $d^{(\log-\det)}$ | $d^{(\mathrm{NSD})}$ | $S_{(\log-\det,\log-\mathrm{MI}}$ |
| 1 | Hydromantes brunus | Oedipina poelzi | Batrachuperus yenyuanensis | Xenopus (sil.) tropicalis | (12)(34) | [31] | • | (13)(24) | • | 0.02343 |
| 2 | Hydromantes brunus | Paramesotriton hongkongensis | Batrachuperus yenyuanensis | Alytes obstetricans pertinax | (12)(34) | [31] | (14)(23) | (13)(24) | (14)(23) | 0.02340 |
| 3 | Plethodon cinereus | Desmognathus fuscus | Ranodon sibiricus | Typhlonectes natans | (12)(34) | [31] | • | (14)(23) | • | 0.02308 |
| 4 | Eurycea bislineata | Gyrinophilus porphyriticus | Desmognathus fuscus | Xenopus (sil.) tropicalis | (12)(34) | [31] | • | (13)(24) | • | 0.02265 |
| 5 | Hydromantes brunus | Oedipina poelzi | Pachyhynobius shangchengensis | Bufo gargarizans | (12)(34) | [31] | • | (13)(24) | (14)(23) | 0.02196 |
| 6 | Ranodon sibiricus | Xenopus (sil.) tropicalis | Scolecomorphus vittatus | Typhlonectes natans | (12)(34) | [31] | • | (13)(24) | (14)(23) | 0.02093 |
| 7 | Bufo gargarizans | Pachyhynobius shangchengensis | Scolecomorphus vittatus | Typhlonectes natans | (12)(34) | [31] | • | (14)(23) | (13)(24) | 0.02080 |
| 8 | Plethodon cinereus | Desmognathus wrighti | Ichthyophis glutinosus | Typhlonectes natans | (12)(34) | [31] | • | (13)(24) | • | 0.01940 |
| 9 | Ranodon sibiricus | Xenopus (sil.) tropicalis | Scolecomorphus vittatus | Rhinatrema bivittatum | (12)(34) | [31] | • | (14)(23) | (13)(24) | 0.01889 |
| 10 | Oedipina poelzi | Thorius n. sp. RLM-2004 | Pseudotriton ruber | Gegeneophis ramaswamii | (12)(34) | [32] | (14)(23) | • | (14)(23) | 0.01684 |

TABLE V: Same as Table I, but for amphibia.

| nematoda | | | | | | | | | | |
|---|---|---|---|---|---|---|---|---|---|---|
| | species names | | | | | | classification predicted by | | | |
| Nr. | species 1 | species 2 | species 3 | species 4 | "true" | Ref. | $d^{(\log-\mathrm{MI})}$ | $d^{(\log-\det)}$ | $d^{(\mathrm{NSD})}$ | $S_{(\log-\det,\log-\mathrm{MI})}$ |
| 1 | Metastrongylus salmi | Trichostrongylus vitrinus | Toxocara malaysiensis | Caenorhabditis elegans | (12)(34) | [25, 27] | • | (13)(24) | • | 0.05208 |
| 2 | Metastrongylus salmi | Trichostrongylus vitrinus | Toxocara canis | Caenorhabditis elegans | (12)(34) | [25, 27] | • | (13)(24) | • | 0.04941 |
| 3 | Metastrongylus salmi | Mecistocirrus digitatus | Toxocara malaysiensis | Caenorhabditis elegans | (12)(34) | [25, 27] | • | (13)(24) | • | 0.04938 |
| 4 | Steinernema carpocapsae | Angiostrongylus cantonensis | Ascaris suum | Caenorhabditis elegans | ? | – | (13)(24) | (14)(23) | (13)(24) | 0.04833 |
| 5 | Mecistocirrus digitatus | Metastrongylus salmi | Toxocara cati | Caenorhabditis elegans | (12)(34) | [25, 27] | • | (14)(23) | • | 0.04296 |
| 6 | Metastrongylus salmi | Cylicocyclus insignis | Toxocara canis | Caenorhabditis elegans | (12)(34) | [25, 27] | • | (13)(24) | • | 0.04269 |
| 7 | Metastrongylus salmi | Ancylostoma caninum | Toxocara canis | Caenorhabditis elegans | (12)(34) | [25, 27] | • | (13)(24) | • | 0.04269 |
| 8 | Trichostrongylus vitrinus | Angiostrongylus cantonensis | Toxocara canis | Caenorhabditis elegans | (12)(34) | [25, 27] | • | (14)(23) | • | 0.04196 |
| 9 | Teladorsagia circumcincta | Angiostrongylus costaricensis | Toxocara canis | Caenorhabditis elegans | (12)(34) | [25, 27] | • | (14)(23) | • | 0.03318 |
| 10 | Metastrongylus salmi | Necator americanus | Toxocara cati | Caenorhabditis elegans | (12)(34) | [25, 27] | • | (13)(24) | • | 0.03301 |
| 11 | Teladorsagia circumcincta | Metastrongylus salmi | Toxocara cati | Caenorhabditis elegans | (12)(34) | [25, 27] | • | (14)(23) | • | 0.03248 |
| 12 | Chabertia ovina | Strongylus vulgaris | Cooperia oncophora | Angiostrongylus cantonensis | (12)(34) | [27, 33] | • | (13)(24) | • | 0.03171 |
| 13 | Strongylus vulgaris | Oesophagostomum dentatum | Ascaris suum | Trichostrongylus vitrinus | (12)(34) | [33] | • | (13)(24) | • | 0.03113 |

TABLE VI: Same as Table I, but for nematoda.

| crustacea | | | | | | | | | | |
|---|---|---|---|---|---|---|---|---|---|---|
| | species names | | | | | | classification predicted by | | | |
| Nr. | species 1 | species 2 | species 3 | species 4 | "true" | Ref. | $d^{(\log-\mathrm{MI})}$ | $d^{(\log-\det)}$ | $d^{(\mathrm{NSD})}$ | $S_{(\log-\det,\log-\mathrm{MI})}$ |
| 1 | Harpiosquilla harpax | Squilla mantis | Halocaridina rubra | Callinectes sapidus | (12)(34) | [25, 27] | (14)(23) | • | (14)(23) | 0.01691 |
| 2 | Macrobrachium rosenbergii | Scylla tranquebarica | Marsupenaeus japonicus | Marsupenaeus japonicus | (12)(34) | [25, 27] | • | (14)(23) | • | 0.01483 |
| 3 | Exopalaemon carinicauda | Scylla tranquebarica | Gonodactylus chiragra | Litopenaeus vannamei | (12)(34) | [25, 27] | • | (13)(24) | • | 0.01466 |
| 4 | Callinectes sapidus | Charybdis japonica | Portunus trituberculatus | Pseudocarcinus gigas | (12)(34) | [34] | • | (13)(24) | • | 0.01447 |
| 5 | Litopenaeus vannamei | Charybdis japonica | Squilla mantis | Daphnia pulex | (12)(34) | [25, 27] | (13)(24) | • | (13)(24) | 0.01435 |
| 6 | Exopalaemon carinicauda | Portunus trituberculatus | Fenneropenaeus chinensis | Lysiosquillina maculata | (12)(34) | [25, 27] | (13)(24) | • | (13)(24) | 0.02397 |
| 7 | Portunus trituberculatus | Litopenaeus vannamei | Squilla mantis | Daphnia pulex | (12)(34) | [25, 27] | (13)(24) | • | (13)(24) | 0.01356 |

TABLE VII: Same as Table I, but for crustacea.

| mollusca | | | | | | | | | | |
|---|---|---|---|---|---|---|---|---|---|---|
| | species names | | | | | | classification predicted by | | | |
| Nr. | species 1 | species 2 | species 3 | species 4 | "true" | Ref. | $d^{(\log-\mathrm{MI})}$ | $d^{(\log-\det)}$ | $d^{(\mathrm{NSD})}$ | $S_{(\log-\det,\log-\mathrm{MI})}$ |
| 1 | Lophiotoma cerithiformis | Terebra dimidiata | Nassarius reticulatus | Conus textile | (12)(34) | [35] | • | (13)(24) | • | 0.02338 |
| 2 | Ascobulla fragilis | Elysia chlorotica | Biomphalaria tenagophila | Onchidella celtica | (12)(34) | [27, 36] | • | (13)(24) | • | 0.02090 |
| 3 | Biomphalaria tenagophila | Siphonaria pectinata | Ascobulla fragilis | Terebra dimidiata | ? | [27, 36] | (14)(23) | (13)(24) | (14)(23) | 0.01933 |
| 4 | Lophiotoma cerithiformis | Terebra dimidiata | Nassarius reticulatus | Conus borgesi | (12)(34) | [35] | • | (13)(24) | • | 0.01892 |
| 5 | Fusiturris similis | Terebra dimidiata | Cymatium parthenopeum | Conus textile | (12)(34) | [35] | • | (14)(23) | • | 0.01817 |
| 6 | Ilyanassa obsoleta | Terebra dimidiata | Cancellaria cancellata | Oncomelania hupensis | (12)(34) | [37] | • | (14)(23) | • | 0.01773 |
| 7 | Terebra dimidiata | Rapana venosa | Oncomelania hup. robertsoni | Cancellaria cancellata | (12)(34) | [37] | • | (14)(23) | • | 0.01656 |
| 8 | Ascobulla fragilis | Aplysia californica | Biomphalaria tenagophila | Pupa strigosa | (12)(34) | [37] | • | (13)(24) | • | 0.01616 |

TABLE VIII: Same as Table I, but for mollusca.

| platyhelminthes | | | | | | | | | | |
|---|---|---|---|---|---|---|---|---|---|---|
| | species names | | | | | | classification predicted by | | | |
| Nr. | species 1 | species 2 | species 3 | species 4 | "true" | Ref. | $d^{(\log-\mathrm{MI})}$ | $d^{(\log-\det)}$ | $d^{(\mathrm{NSD})}$ | $S_{(\log-\det,\log-\mathrm{MI})}$ |
| 1 | Taenia pisiformis | Taenia crassiceps | Echinococcus oligarthrus | Hymenolepsis diminuta | (12)(34) | [38] | (14)(23) | • | (14)(23) | 0.02330 |
| 2 | Taenia pisiformis | Taenia asiatica | Echinococcus canadensis | Taenia crassiceps | (12)(34) | [38, 39] | (13)(24) | (14)(23) | (13)(24) | 0.01957 |
| 3 | Taenia pisiformis | Taenia crassiceps | Echinococcus multilocularis | Hymenolepsis diminuta | (12)(34) | [38] | (14)(23) | • | (14)(23) | 0.01930 |
| 4 | Taenia pisiformis | Taenia crassiceps | Spirometra erinaceieuropaei | Echinococcus vogeli | (12)(34) | [38] | (13)(24) | • | • | 0.01831 |
| 5 | Taenia pisiformis | Taenia asiatica | Taenia crassiceps | Echinococcus vogeli | (12)(34) | [38, 39] | • | (13)(24) | • | 0.01734 |
| 6 | Taenia pisiformis | Taenia multiceps | Taenia hydatagenia | Echinococcus shiquicus | (12)(34) | [39] | (14)(23) | • | (14)(23) | 0.01625 |
| 7 | Taenia pisiformis | Taenia saginata | Echinococcus multilocularis | Diphyllobothrium latum | (12)(34) | [38] | • | (14)(23) | • | 0.01174 |
| 8 | Echinococcus multilocularis | Echinococcus granulosus | Echinococcus oligarthrus | Taenia asiatica | (12)(34) | [40] | • | (14)(23) | • | 0.00998 |

TABLE IX: Same as Table I, but for platyhelminthes.

| | U. maritimus | U. americanus | U. thibetanus | O. cuniculus |
|---|---|---|---|---|
| | $d^{(NSD)}$ | | | |
| U. maritimus | – | 0.23364 | 0.21966 | 0.59586 |
| U. americanus | 0.23444 | – | 0.19891 | 0.57536 |
| U. thibetanus | 0.21851 | 0.19539 | – | 0.58062 |
| O. cuniculus | 0.59586 | 0.57536 | 0.58062 | – |
| | $d^{(\log-\mathrm{MI})}$ | | | |
| U. maritimus | – | 0.26611 | 0.24802 | 0.90600 |
| U. americanus | 0.26611 | – | 0.22178 | 0.85651 |
| U. thibetanus | 0.24802 | 0.22178 | – | 0.86897 |
| O. cuniculus | 0.90600 | 0.86897 | 0.86897 | – |

TABLE X: Two distance matrices for the same quartet obtained with the normalized Shannon distance (top) and with its log-transformed version (bottom). With the first, one obtains the wrong classification ((*americanus, thibetanus*), *maritimus*) due to the Felsenstein phenomenon, since $d^{(\mathrm{NSD})}$ is not additive. With the second, additivity is approximately restored, but noise is amplified, resulting in the wrong classification ((*maritimus, thibetanus*), *americanus*). The correct classification would be [41] ((*maritimus, americanus*), *thibetanus*).
